# Supplementary material for: Experimental assessment of mixing layer scaling laws in Rayleigh-Taylor instability
Source: arXiv:2206.13363 ancillary file (2022-09-17)
Supplement: Supplementary file 1 [file supplemental_information.pdf]

# Experimental assessment of mixing layer scaling laws in Rayleigh-Taylor instability (Supplemental information)

Marco De Paoli,[1,2,*] Diego Perissutti,[3] Cristian Marchioli,[3] and Alfredo Soldati[1,3]

[1] *Institute of Fluid Mechanics and Heat Transfer, TU Wien, 1060 Vienna, Austria*
[2] *Physics of Fluids Group, University of Twente, 7500AE Enschede, The Netherlands*
[3] *Polytechnic Department, University of Udine, 33100 Udine, Italy*

(Dated: June 25, 2022)

**Content of this file**
Image processing and correction techniques are here presented. We describe the effect of the image processing algorithms applied to improve the quality of the measurements performed, which consist of three main steps: noise filtering (Sec. S.1), non-uniform light intensity correction (Sec. S.2) and image rotation (Sec. S.3).

**Additional supporting information**

A. Caption for "Movie S1"
B. Caption for "Movie S2"

## S.1. Noise filtering

Images are affected by both noise and disturbances, such as dust particles or small bubbles, which cause non-physical discontinuities in the detected concentration field. Traditional filtering techniques (e.g. Gaussian or median filters) are not effective in this case, due to the physical discontinuities that characterize the interface between the two fluid regions in the early stages of the phenomenon. In fact, a Gaussian or a median filter produce an undesired reduction of the resolution in correspondence of the interface. In contrast, a sharp spectral low-pass filter would cause non-physical overshoots in the concentration field. To overcome these limitations, we employed an algorithm detecting disturbances in the light intensity distributions.

The filtering method used is applied to sub-windows (size $8 \times 8$ pixel) of the reconstructed concentration field, and consist of several steps:

i) computing the variance of the concentration field within the subset of the image (window) considered;

ii) comparing the value in each window against the values in the neighbour windows;

iii) if the variance exceeds a certain threshold (which has been defined as 8 times the average variance of the neighbour windows) it imposes the concentration field to be equal to the mean value of the neighbour windows.

We observed that the application of the present filtering method reduces remarkably the presence of isolated light intensity spots in the bulk of the domain, e.g. when the fluid is initially characterised by large regions with uniform concentration.

* Author to whom correspondence should be addressed: marco.de.paoli@tuwien.ac.at

## S.2. Non-uniform light intensity correction

A uniform cell illumination (i.e., a uniform distribution of the light intensity over the cell), is crucial to determine global and local flow quantities. These effects in the present configuration have been quantified here [1]. However, due to non-ideal experimental conditions, the light intensity over the cell is not uniform. Both the finite extension of the illumination system and the shadow generated by the cell boundaries contribute to this undesired effect, which generates a space-dependent $(x^*, z^*)$ disturbance affecting the measurements of the concentration field. To compensate for this disturbance, we developed an algorithm which corrects the light intensity distribution of the acquired images. The algorithm provides a function that correlates the corrected light intensity value ($I$) to the detected light intensity value ($I_m$) and the dimensionless horizontal and vertical spacial coordinates $(x^*, z^*)$, both defined in the interval $[0;Ra]$.

We assume that $I(x^*, z^*)$ is only affected by the local solute concentration, $C^*(x^*, z^*)$. Therefore by applying the function to a calibration image, a nearly uniform corrected light intensity field $I(x^*, z^*)$ is obtained. We also assume that the shadow disturbance depends only on the spatial position and the local concentration value (i.e. the local corrected light intensity value $I$). The algorithm uses numerical coefficients derived by interpolating light intensity fields obtained from calibration images with quadratic functions of $\tilde{x} = x^*/Ra$ and $\tilde{z} = z^*/Ra$, which are the horizontal and vertical normalized coordinates (both 0 on the bottom left corner of the calibration images and 1 on the top right). The chosen quadratic functions are

$$g_x(\tilde{x}) = a_x\tilde{x}^2 + b_x\tilde{x} + c_x \tag{S1}$$

$$g_z(\tilde{z}) = a_z\tilde{z}^2 + b_z\tilde{z} + c_z. \tag{S2}$$

The coefficients $a_x$, $b_x$, $c_x$, $a_z$, $b_z$, $c_z$ are found by interpolating the horizontal and vertical mean light intensity

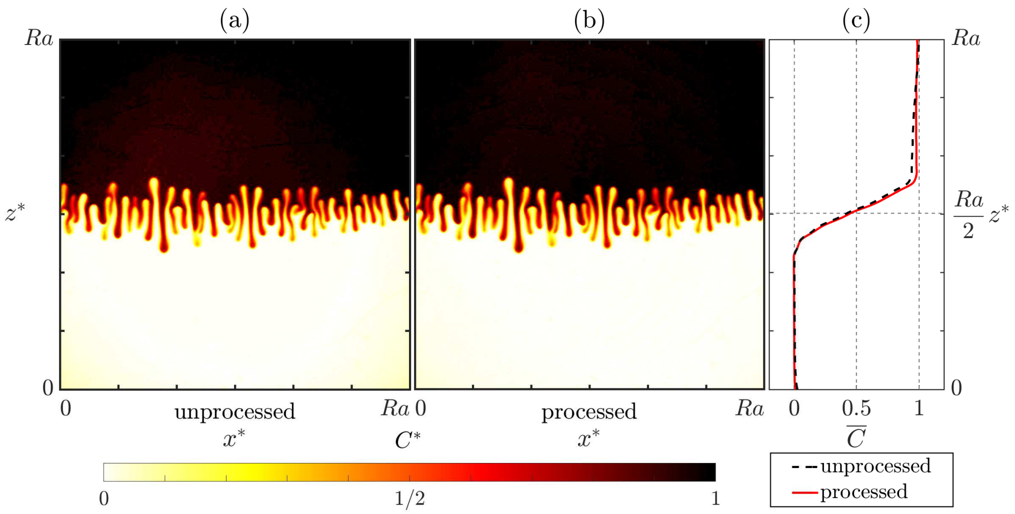


FIG. S1. Concentration field before (a) and after (b) the shadow correction algorithm. The correction is evident at the lower corners of the cells, which present in (a) a non uniform concentration. After correction, the differences with the nearby regions are reduced. A quantitative estimate of the effect of the correction is provided in (c), where the horizontally-averaged concentration profiles [Eq. (18)] are reported. One can observe that the unprocessed data exhibit a value of concentration, which is not uniform along $z^*$ also outside of the mixing region (dashed line). After the correction is applied (solid line), the profiles is nearly uniform and the concentration outside of the mixing region attains the values expected ($C = 0$ for $z^* < Ra/2$, $C = 1$ for $z^* > Ra/2$).

profile of a given calibration image, such that

$$g_x(\tilde{x}, \langle I_m^{cal} \rangle) \approx \int_0^1 I_m^{cal}(\tilde{x}, \tilde{z}) d\tilde{z} \tag{S3}$$

$$g_z(\tilde{z}, \langle I_m^{cal} \rangle) \approx \int_0^1 I_m^{cal}(\tilde{x}, \tilde{z}) d\tilde{x}. \tag{S4}$$

where $I_m^{cal}$ is the light intensity field of a calibration image detected by the camera and $\langle \cdot \rangle$ indicates average of the entire field. This algorithm exploits the similarity of the horizontal and vertical light intensity fields sections to provide a function, $f$, that approximates well the two-dimensional field without much computational effort. This function is defined from $g_x$ and $g_z$ as

$$f(\tilde{x}, \tilde{z}) = \frac{g_x(\tilde{x}) g_z(\tilde{z})}{\bar{g}}, \tag{S5}$$

where

$$\bar{g}(I) = \frac{1}{2} \left( \int_0^1 g_z(\tilde{z}) d\tilde{z} + \int_0^1 g_x(\tilde{x}) d\tilde{x} \right). \tag{S6}$$

For all detected calibration light intensity fields $I_{m,i}^{cal}$, the interpolation process provides a set of coefficients $a_{x,i}$, $b_{x,i}$, $c_{x,i}$, $a_{z,i}$, $b_{z,i}$, $c_{z,i}$ and an approximating function $f_i(\tilde{x}, \tilde{z})$. The objective is to associate each of this functions to a constant corrected light intensity value $I$, which for this case has been defined as the average detected light intensity field of the calibration image $\langle I_{m,i}^{cal} \rangle$. Each coefficient is then expressed as a piecewise-linear function of the corrected light intensity value $I$ by interpolating the point values derived by the association already defined. By plugging these new coefficients expressed as function of $I$ into the definition (S5), a function $f(\tilde{x}, \tilde{z}, I)$ which depends also on $I$ is provided. Using this definition and the previous assumptions, it holds

$$f(\tilde{x}, \tilde{z}, \langle I_{m,i}^{cal} \rangle) \approx I_{m,i}^{cal}. \tag{S7}$$

Therefore, because of the assumption made, it is possible to claim that $f$ approximates the detected light intensity field. Moreover, at a given spatial point, it is possible to express $f$ as a quadratic function of $I$. Thus, in every interval for $I$ of the piece-wise linear functions that express the set of coefficients,

$$I_m(\tilde{x}, \tilde{z}) \approx A(\tilde{x}, \tilde{z}) I^2 + B(\tilde{x}, \tilde{z}) I + C(\tilde{x}, \tilde{z}), \tag{S8}$$

with $A$, $B$ and $C$ depending on the spatial coordinates and on the slope of the piecewise linear functions. This function is computationally easy to invert in order to get the corrected field $I(\tilde{x}, \tilde{z})$ from the detected light intensity $I_m(\tilde{x}, \tilde{z})$. This function is then applied to all points of raw images acquired during experimental runs in order to correct them. The benefits of the correction applied are apparent, particularly at the corners of the cell, where the light intensity distribution is more heterogeneous than in other parts. An example of the effects of the correction proposed in shown Fig. S1, where a concentration field is shown before (Fig. S1a) and after (Fig. S1b) the shadow correction algorithm is applied. After correction, the differences between the concentration at the corners with respect to the nearby regions are reduced. A quantita-

tive estimate of the effect of the correction is provided in Fig. S1(c), where the horizontally-averaged concentration profiles are reported. One can observe that the unprocessed data exhibit a value of concentration, which is not uniform along $z^*$ also outside of the mixing region (dashed line). After the correction is applied (solid line), the profile is nearly uniform and the concentration outside of the mixing region attains the expected values ($C = 0$ for $z^* < Ra/2$, $C = 1$ for $z^* > Ra/2$). We refer to [1, 2] for further details on the process of calibration.

### S.3. Image rotation

Another source of disturbance is the possible misalignment of the camera in the experimental setup. For this reason, the interface between the two fluid regions in the initial phase might not appear horizontal in the image. To correct this error, and thus making data processing easier, we developed an algorithm that rotates the image in order to obtain an horizontal interface. The algorithm detects first the initial position of the interface as the longest contour line corresponding to the mean value of the dimensionless concentration field, $C^* = 0.5$. Then it interpolates the points of the detected interface with a linear function, and it rotates the image by an angle that is defined based on the slope of the linear interpolation. We observed that the uncertainty on the alignment of the camera with respect to cell frame is always $\leq 1.5°$. However, these small deviations can produce a visible difference in the measurement of some relevant flow features, e.g. the early stage evolution of the mixing length.

## Additional supporting information

### A. Caption for "Movie S1"

Time-dependent evolution of dimensionless concentration field ($C^*$) obtained experimentally ($Ra = 19789$, left) and numerically (De Paoli *et al.*, Phys. Rev. Fluids, **4**, 023502 (2019), [3], $Ra = 19953$, right) The dimensionless ($t^*$) and corresponding dimensional ($t$) time instants at which the fields refer are explicitly indicated. Note that dimensionless experimental domain size is $Ra \times Ra$, whereas this simulation is performed in a domain of size $\pi Ra/4 \times Ra$. Therefore, for better comparison, only a portion of the experimental domain is shown.

### B. Caption for "Movie S2"

Time-dependent evolution of the fingers number and corresponding concentration field for $Ra = 5.43 \times 10^4$. The dimensionless concentration field ($C^*$) and the space-time map, consisting of the evolution of the concentration field along the centerline, $C^*(x^*, z^* = Ra/2, t^*)$, are shown. To compute the finger number, the space-time map is binarized, $\widehat{C}(x^*, z^* = Ra/2, t^*)$, choosing $C^* = 1/2$ as threshold. The concentration profile (red solid line) and the discretized profile (white solid line) measured along the centerline at $t^* \approx 1.1 \times 10^5$ are also reported as a function of the horizontal coordinate $x^*$. Finally, the time-dependent finger number is computed as from the binarized field $\widehat{C}$ (white line) and from power-averaged mean wavenumber as defined in Eq. (21) ($\langle N \rangle = L\langle k \rangle/\pi$, red line).

[1] M. Alipour and M. De Paoli. Convective dissolution in porous media: Experimental investigation in Hele-Shaw cell. *PAMM*, 19(1):e201900236, 2019.

[2] M. Alipour, M. De Paoli, and A. Soldati. Concentration-based velocity reconstruction in convective Hele–Shaw flows. *Exp. Fluids*, 61(9):1–16, 2020.

[3] M. De Paoli, F. Zonta, and A. Soldati. Rayleigh-Taylor convective dissolution in confined porous media. *Phys. Rev. Fluids*, 4:023502, 2019.
